# Supplementary material for: Neighbor Oblivious Learning (NObLe) for Device Localization and Tracking
Source: arXiv:2011.14954 source file (2020-11-23)
Supplement: Supplementary file 1 [file appendix.tex]

\begin{appendices}

\section{Datasets for \wifi Localization}
Two publicly available \wifi \fp datasets: IPIN2016~\cite{Sansano2016} and  UJIIndoorLoc~\cite{8767421} were used for \wifi localization. These two dataset can be downloaded from UCI repository. IPIN2016, which is created for the \fp-based indoor position tutorial in the International Conference on Indoor Positioning and Indoor Navigation. The dataset covers an area of 6 by 31 meters with 168 WAPs. It contains 927 data points and we reserve 185 points for testing purpose. UJIIndoorLoc covers three buildings, 4 floors, and a space of 397 by 273 meters with 520 WAPs. It contains 19,937 training instances for which 3,987 instances are reserved for testing. At each sample location, received \wifi signal strength readings were recorded as negative integer values, and positive 100 is used when a WAP is not detected.  In addition to exact coordinates, IPIN2016 contains space information, representing sub-spaces such as classrooms, offices, etc. We use space class and cell class as labels for our experiment on IPIN2016\_tutorial. UJIIndoorLoc contains building, floor, and space information. We use building, floor, space ID, and cell ID as labels for our experiment on UJIIndoorLoc. 

\section{Dataset for IMU Tracking}
The original dataset was collected over Academic Quad of Rice University (160 meters $\times$ 60 meters) and contains ten components: 3 axis gyroscope, 3-axis accelerometer, location based GPS coordinates, and timestamps. There are in total 177 sample points with coordinates, and between each sample points, there are 768 readings for each inertial sensor on a single axis. We set the maximum sample point on a single path to be 50 and we construct our path dataset as follows: (1) randomly choose a sample point as start position, (2) randomly choose a path length less than 50 and determine the end position according to the randomized path length, (3) concatenate IMU readings between starting and ending positions as the input to our model. In total, we obtained 6,857 path data. We use 4,389 paths as training, 1,096 paths as validation and 1,372 paths for testing,

\end{appendices}
